# Supplementary material for: High-resolution momentum distributions from low-resolution wave functions
Source: arXiv:2402.00634 ancillary file (2024-04-11)
Supplement: Supplementary file 1 [file supplemental.pdf]

# Supplemental material

A. J. Tropiano[1], S. K. Bogner[2], R. J. Furnstahl[3],

M. A. Hisham[3], A. Lovato[1,4], R. B. Wiringa[1]

[1] *Physics Division, Argonne National Laboratory, Argonne, IL 60439, USA*

[2] *Facility for Rare Isotope Beams and Department of Physics and Astronomy, Michigan State University, East Lansing, MI 48824, USA*

[3] *Department of Physics, The Ohio State University, Columbus, OH 43210, USA*

[4] *Computational Science Division, Argonne National Laboratory, Argonne, IL, 60439, USA*

(Dated: February 7, 2024)

## I. ADDITIONAL FIGURES

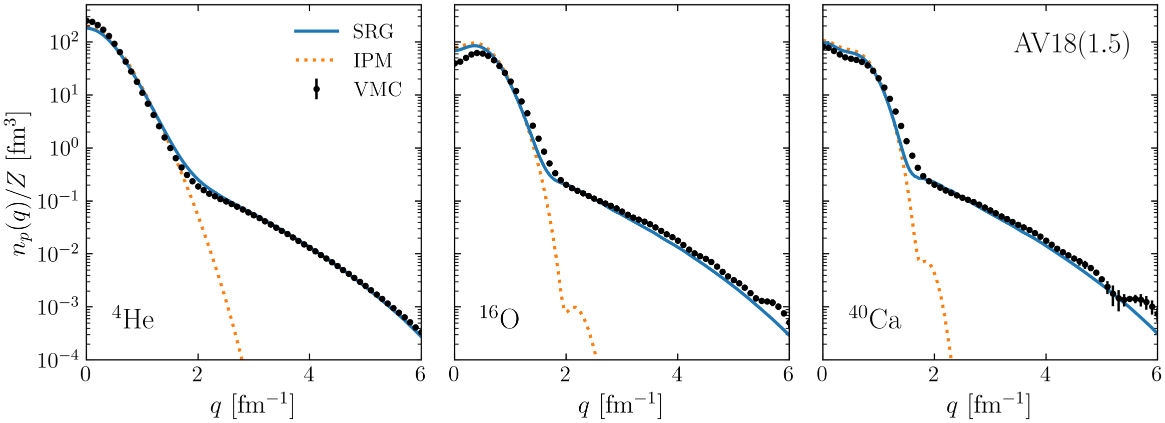


FIG. 1. Proton momentum distributions for $^4$He, $^{16}$O, and $^{40}$Ca. The solid blue lines show the SRG distributions in which the operator is evolved under the AV18 interaction at $\lambda = 1.5\,\text{fm}^{-1}$. The dashed orange lines show the IPM distributions (no operator evolution). The black points show the VMC distribution for $^4$He and CVMC distributions for $^{16}$O and $^{40}$Ca, all calculated using AV18 and no three-nucleon interaction. Each distribution is divided by the proton number $Z$.

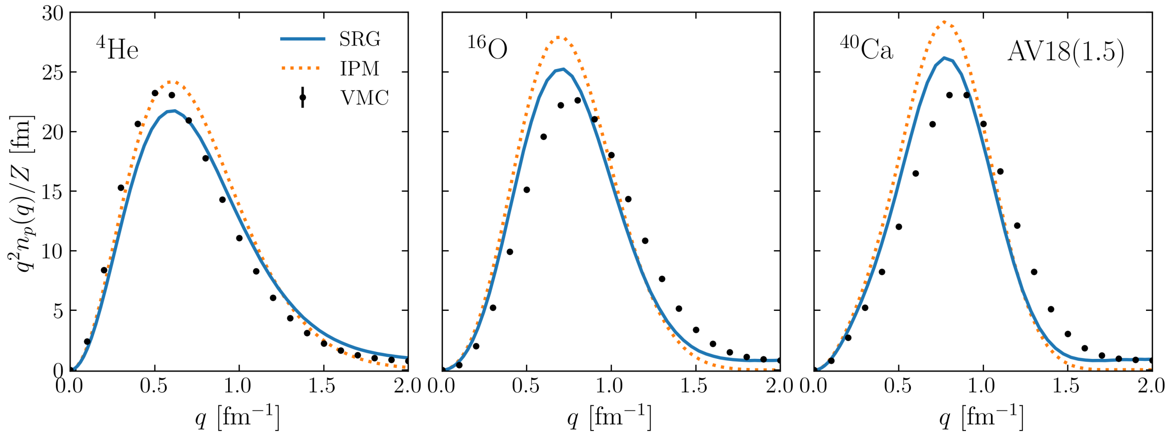


FIG. 2. Same as Fig. 1 but on a linear y-scale with a factor of $q^2$ included.

Figures 1 and 2 show SRG proton momentum distributions of $^4$He, $^{16}$O, and $^{40}$Ca using AV18 with $\lambda = 1.5\,\text{fm}^{-1}$ compared to VMC and CVMC results with AV18 and no three-nucleon interaction. The same Woods-Saxon potential is used for the SRG distributions shown here as the analogous SRG distributions shown in the paper. This Woods-Saxon parametrization was adjusted to match VMC and CVMC results that include a three-nucleon

interaction. Table I compares point RMS proton radii obtained from various Woods-Saxon parametrizations to VMC, CVMC, and experiment.

TABLE I. Point RMS proton radii for $^4$He, $^{12}$C, $^{16}$O, and $^{40}$Ca in units fm$^{-1}$. We compare radii obtained from various Woods-Saxon parametrizations to VMC, CVMC, and experiment [1]. We show three different Woods-Saxon parametrizations, where "Match" corresponds to the parametrization used for matching to VMC or CVMC distributions. For VMC and CVMC we use different combinations of AV18, UIX, and UX indicated by the column, where $^4$He and $^{12}$C radii are calculated with VMC and $^{16}$O and $^{40}$Ca radii are calculated with CVMC.

| Nucleus | Universal | Seminole | Match | AV18 | AV18 + UIX | AV18 + UX | Experimental |
|---|---|---|---|---|---|---|---|
| $^4$He | 2.30 | 1.84 | 1.87 | 1.52 | | 1.44 | 1.46 |
| $^{12}$C | 2.67 | 2.42 | 2.48 | | 2.35 | 2.35 | 2.33 |
| $^{16}$O | 2.76 | 2.56 | 2.83 | 2.40 | 2.62 | | 2.57 |
| $^{40}$Ca | 3.47 | 3.33 | 3.72 | 3.26 | 3.53 | | 3.38 |

## II. SINGLE-NUCLEON MOMENTUM DISTRIBUTION DERIVATION

The single-nucleon momentum distribution at high and low resolution are given by matrix elements in the $A$-nucleon ground state $\left|\Psi_0^A\right\rangle$,

$$\begin{aligned}\left\langle\Psi_0^A\middle|\widehat{n}_\infty^\tau(\mathbf{q})\middle|\Psi_0^A\right\rangle &= \left\langle\Psi_0^A\middle|\widehat{U}_\lambda^\dagger\widehat{U}_\lambda\widehat{n}_\infty^\tau(\mathbf{q})\widehat{U}_\lambda^\dagger\widehat{U}_\lambda\middle|\Psi_0^A\right\rangle \\ &\equiv \left\langle\Psi_0^A(\lambda)\middle|\widehat{n}_\lambda^\tau(\mathbf{q})\middle|\Psi_0^A(\lambda)\right\rangle, \end{aligned} \tag{1}$$

where SRG transformations $\widehat{U}_\lambda$ are applied to both the wave function and operator [2] (after which they are labeled by $\lambda$). The initial operator and evolved operators are given in second quantization by

$$\widehat{n}_\infty^\tau(\mathbf{q}) = \sum_\sigma a^\dagger_{\mathbf{q}\sigma\tau}a_{\mathbf{q}\sigma\tau}, \tag{2}$$

$$\widehat{n}_\lambda^\tau(\mathbf{q}) = \widehat{U}_\lambda\widehat{n}_\infty^\tau(\mathbf{q})\widehat{U}_\lambda^\dagger, \tag{3}$$

where $\mathbf{q}$ is the single-nucleon momentum, $\sigma$ is the spin projection, and $\tau$ is the isospin projection. The subscript of the operator indicates whether it is SRG-evolved or not ($\lambda = \infty$

is unevolved). The SRG unitary transformation at flow parameter $\lambda$ in the plane-wave basis is given by

$$\widehat{U}_\lambda = \widehat{I} + \frac{1}{4} \sum_{\sigma_1\sigma_2\sigma_3\sigma_4} \sum_{\tau_1\tau_2\tau_3\tau_4} \int d\mathbf{K} \int d\mathbf{k} \int d\mathbf{k}' (\mathbf{k}\sigma_1\tau_1\sigma_2\tau_2 | \delta U_\lambda | \mathbf{k}'\sigma_3\tau_3\sigma_4\tau_4)$$
$$\times\, a^\dagger_{\frac{1}{2}\mathbf{K}+\mathbf{k}\sigma_1\tau_1} a^\dagger_{\frac{1}{2}\mathbf{K}-\mathbf{k}\sigma_2\tau_2} a_{\frac{1}{2}\mathbf{K}-\mathbf{k}'\sigma_4\tau_4} a_{\frac{1}{2}\mathbf{K}+\mathbf{k}'\sigma_3\tau_3} + \ldots, \tag{4}$$

where $\mathbf{k}$ and $\mathbf{k}'$ are relative momenta, $\mathbf{K}$ is the total momentum, and the rounded brackets indicate an antisymmetrized matrix element. Equations up to this point are exact. In the following sections, we derive the momentum distribution by truncating three-body and higher induced operators in evaluating Eq. (3), and replace the fully evolved ground state $|\Psi_0^A(\lambda)\rangle$ by a single Slater determinant of Woods-Saxon orbitals, after which Eq. (1) is no longer exact.

### A. SRG-evolved operator

We apply SRG transformations to the initial momentum distribution operator (2) and use Wick's theorem in operator form to truncate at the two-body (vacuum) level omitting three-body and higher-body operators of Eq. (4). The operator $\widehat{U}_\lambda \widehat{n}^\tau_\infty(\mathbf{q}) \widehat{U}^\dagger_\lambda$ has four terms at the two-body level:

- $\widehat{I}\widehat{n}^\tau_\infty(\mathbf{q})\widehat{I}$
- $\delta\widehat{U}_\lambda\widehat{n}^\tau_\infty(\mathbf{q})\widehat{I}$
- $\widehat{I}\widehat{n}^\tau_\infty(\mathbf{q})\delta\widehat{U}^\dagger_\lambda$
- $\delta\widehat{U}_\lambda\widehat{n}^\tau_\infty(\mathbf{q})\delta\widehat{U}^\dagger_\lambda$

where $\delta\widehat{U}_\lambda$ represents the second term in Eq. (4). The first term is simple because the initial operator is unchanged

$$\widehat{I}\widehat{n}^\tau_\infty(\mathbf{q})\widehat{I} = \sum_\sigma a^\dagger_{\mathbf{q}\sigma\tau} a_{\mathbf{q}\sigma\tau}. \tag{5}$$

The second term is

$$
\begin{aligned}
\delta\widehat{U}_\lambda \widehat{n}^\tau(\mathbf{q})\widehat{I} &= \frac{1}{4}\sum_{\sigma_1\sigma_2\sigma_3\sigma_4\sigma}\sum_{\tau_1\tau_2\tau_3\tau_4}\int d\mathbf{K}\int d\mathbf{k}\int d\mathbf{k}'(\mathbf{k}\sigma_1\tau_1\sigma_2\tau_2|\delta U_\lambda|\mathbf{k}'\sigma_3\tau_3\sigma_4\tau_4) \\
&\quad\times a^\dagger_{\frac{1}{2}\mathbf{K}+\mathbf{k}\sigma_1\tau_1} a^\dagger_{\frac{1}{2}\mathbf{K}-\mathbf{k}\sigma_2\tau_2} a_{\frac{1}{2}\mathbf{K}-\mathbf{k}'\sigma_4\tau_4} a_{\frac{1}{2}\mathbf{K}+\mathbf{k}'\sigma_3\tau_3} a^\dagger_{\mathbf{q}\sigma\tau} a_{\mathbf{q}\sigma\tau} \\
&\approx \frac{1}{4}\sum_{\sigma_1\sigma_2\sigma_3\sigma_4\sigma}\sum_{\tau_1\tau_2\tau_3\tau_4}\int d\mathbf{K}\int d\mathbf{k}\int d\mathbf{k}'(\mathbf{k}\sigma_1\tau_1\sigma_2\tau_2|\delta U_\lambda|\mathbf{k}'\sigma_3\tau_3\sigma_4\tau_4) \\
&\quad\times \big(\overbracket{a_{\frac{1}{2}\mathbf{K}+\mathbf{k}'\sigma_3\tau_3} a^\dagger_{\mathbf{q}\sigma\tau}} a^\dagger_{\frac{1}{2}\mathbf{K}+\mathbf{k}\sigma_1\tau_1} a^\dagger_{\frac{1}{2}\mathbf{K}-\mathbf{k}\sigma_2\tau_2} a_{\frac{1}{2}\mathbf{K}-\mathbf{k}'\sigma_4\tau_4} a_{\mathbf{q}\sigma\tau} \\
&\qquad - \overbracket{a_{\frac{1}{2}\mathbf{K}-\mathbf{k}'\sigma_4\tau_4} a^\dagger_{\mathbf{q}\sigma\tau}} a^\dagger_{\frac{1}{2}\mathbf{K}+\mathbf{k}\sigma_1\tau_1} a^\dagger_{\frac{1}{2}\mathbf{K}-\mathbf{k}\sigma_2\tau_2} a_{\frac{1}{2}\mathbf{K}+\mathbf{k}'\sigma_3\tau_3} a_{\mathbf{q}\sigma\tau}\big) \\
&= \frac{1}{4}\sum_{\sigma_1\sigma_2\sigma_3\sigma_4\sigma}\sum_{\tau_1\tau_2\tau_3\tau_4}\int d\mathbf{K}\int d\mathbf{k}\int d\mathbf{k}'(\mathbf{k}\sigma_1\tau_1\sigma_2\tau_2|\delta U_\lambda|\mathbf{k}'\sigma_3\tau_3\sigma_4\tau_4) \\
&\quad\times \big(\delta(\mathbf{K}/2+\mathbf{k}'-\mathbf{q})\delta_{\sigma_3\sigma}\delta_{\tau_3\tau} a^\dagger_{\frac{1}{2}\mathbf{K}+\mathbf{k}\sigma_1\tau_1} a^\dagger_{\frac{1}{2}\mathbf{K}-\mathbf{k}\sigma_2\tau_2} a_{\frac{1}{2}\mathbf{K}-\mathbf{k}'\sigma_4\tau_4} a_{\mathbf{q}\sigma\tau} \\
&\qquad - \delta(\mathbf{K}/2-\mathbf{k}'-\mathbf{q})\delta_{\sigma_4\sigma}\delta_{\tau_4\tau} a^\dagger_{\frac{1}{2}\mathbf{K}+\mathbf{k}\sigma_1\tau_1} a^\dagger_{\frac{1}{2}\mathbf{K}-\mathbf{k}\sigma_2\tau_2} a_{\frac{1}{2}\mathbf{K}+\mathbf{k}'\sigma_3\tau_3} a_{\mathbf{q}\sigma\tau}\big) \\
&= \frac{1}{4}\sum_{\sigma_1\sigma_2\sigma}\sum_{\tau_1\tau_2}\int d\mathbf{K}\int d\mathbf{k} \\
&\quad\times \Big(\sum_{\sigma_4\tau_4}(\mathbf{k}\sigma_1\tau_1\sigma_2\tau_2|\delta U_\lambda|\mathbf{q}-\mathbf{K}/2\sigma\tau\sigma_4\tau_4) a^\dagger_{\frac{1}{2}\mathbf{K}+\mathbf{k}\sigma_1\tau_1} a^\dagger_{\frac{1}{2}\mathbf{K}-\mathbf{k}\sigma_2\tau_2} a_{\mathbf{K}-\mathbf{q}\sigma_4\tau_4} a_{\mathbf{q}\sigma\tau} \\
&\qquad - \sum_{\sigma_3\tau_3}(\mathbf{k}\sigma_1\tau_1\sigma_2\tau_2|\delta U_\lambda|\mathbf{K}/2-\mathbf{q}\sigma_3\tau_3\sigma\tau) a^\dagger_{\frac{1}{2}\mathbf{K}+\mathbf{k}\sigma_1\tau_1} a^\dagger_{\frac{1}{2}\mathbf{K}-\mathbf{k}\sigma_2\tau_2} a_{\mathbf{K}-\mathbf{q}\sigma_3\tau_3} a_{\mathbf{q}\sigma\tau}\Big) \\
&= \frac{1}{2}\sum_{\sigma_1\sigma_2\sigma\sigma'}\sum_{\tau_1\tau_2\tau'}\int d\mathbf{K}\int d\mathbf{k}(\mathbf{k}\sigma_1\tau_1\sigma_2\tau_2|\delta U_\lambda|\mathbf{q}-\mathbf{K}/2\sigma\tau\sigma'\tau') \\
&\quad\times a^\dagger_{\frac{1}{2}\mathbf{K}+\mathbf{k}\sigma_1\tau_1} a^\dagger_{\frac{1}{2}\mathbf{K}-\mathbf{k}\sigma_2\tau_2} a_{\mathbf{K}-\mathbf{q}\sigma'\tau'} a_{\mathbf{q}\sigma\tau},
\end{aligned} \tag{6}
$$

where in the last step we relabeled the spin and isospin projections to combine terms using the antisymmetrized matrix element. The third term is similar

$$
\begin{aligned}
\widehat{I}\widehat{n}^\tau(\mathbf{q})\delta\widehat{U}^\dagger_\lambda &\approx \frac{1}{2}\sum_{\sigma_1\sigma_2\sigma\sigma'}\sum_{\tau_1\tau_2\tau'}\int d\mathbf{K}\int d\mathbf{k}(\mathbf{q}-\mathbf{K}/2\sigma\tau\sigma'\tau'|\delta U^\dagger_\lambda|\mathbf{k}\sigma_1\tau_1\sigma_2\tau_2) \\
&\quad\times a^\dagger_{\mathbf{q}\sigma\tau} a^\dagger_{\mathbf{K}-\mathbf{q}\sigma'\tau'} a_{\frac{1}{2}\mathbf{K}-\mathbf{k}\sigma_2\tau_2} a_{\frac{1}{2}\mathbf{K}+\mathbf{k}\sigma_1\tau_1}.
\end{aligned} \tag{7}
$$

The fourth term initially involve sums over nine (eight) spin (isospin) projections because there are both $\delta\widehat{U}_\lambda$ and $\delta\widehat{U}_\lambda^\dagger$ contributions in addition to the initial sum over $\sigma$.

$$\delta\widehat{U}_\lambda \widehat{n}^\tau(\mathbf{q})\delta\widehat{U}_\lambda^\dagger \equiv \frac{1}{16}\sum_{\sigma_1\sigma_2\sigma_3\sigma_4\sigma_5\sigma_6\sigma_7\sigma_8\sigma}\ \sum_{\tau_1\tau_2\tau_3\tau_4\tau_5\tau_6\tau_7\tau_8}\int d\mathbf{K}\int d\mathbf{k}\int d\mathbf{k}'\int d\mathbf{K}'\int d\mathbf{k}''\int d\mathbf{k}'''$$
$$\times (\mathbf{k}\sigma_1\tau_1\sigma_2\tau_2|\delta U_\lambda|\mathbf{k}'\sigma_3\tau_3\sigma_4\tau_4)(\mathbf{k}''\sigma_5\tau_5\sigma_6\tau_6|\delta U_\lambda^\dagger|\mathbf{k}'''\sigma_7\tau_7\sigma_8\tau_8)$$
$$\times a^\dagger_{\frac{1}{2}\mathbf{K}+\mathbf{k}\sigma_1\tau_1} a^\dagger_{\frac{1}{2}\mathbf{K}-\mathbf{k}\sigma_2\tau_2} a_{\frac{1}{2}\mathbf{K}-\mathbf{k}'\sigma_4\tau_4} a_{\frac{1}{2}\mathbf{K}+\mathbf{k}'\sigma_3\tau_3} a^\dagger_{\mathbf{q}\sigma\tau} a_{\mathbf{q}\sigma\tau}$$
$$\times a^\dagger_{\frac{1}{2}\mathbf{K}'+\mathbf{k}''\sigma_5\tau_5} a^\dagger_{\frac{1}{2}\mathbf{K}'-\mathbf{k}''\sigma_6\tau_6} a_{\frac{1}{2}\mathbf{K}'-\mathbf{k}'''\sigma_8\tau_8} a_{\frac{1}{2}\mathbf{K}'+\mathbf{k}'''\sigma_7\tau_7}. \tag{8}$$

We anticipate that the product of creation and annihilation operators in Eq. (8) will give four terms at the two-body level:

- $a^\dagger a^\dagger a a a^\dagger a a^\dagger a^\dagger a a$
- $a^\dagger a^\dagger a a a^\dagger a a^\dagger a^\dagger a a$
- $a^\dagger a^\dagger a a a^\dagger a a^\dagger a^\dagger a a$
- $a^\dagger a^\dagger a a a^\dagger a a^\dagger a^\dagger a a$

We will use the same approach as before in the $\delta\widehat{U}_\lambda \widehat{n}^\tau(\mathbf{q})\widehat{I}$ term. That is, several spin and isospin projections will be relabeled allowing for combinations of terms using the antisymmetrized $\delta U_\lambda$ and $\delta U_\lambda^\dagger$. Thus, we only need to evaluate the first set of contractions listed above and multiply by four. This gives

$$\delta\widehat{U}_\lambda \widehat{n}^\tau(\mathbf{q})\delta\widehat{U}_\lambda^\dagger = \frac{1}{4}\sum_{\sigma_1\sigma_2\sigma_3\sigma_4\sigma_5\sigma_6\sigma_7\sigma_8\sigma}\ \sum_{\tau_1\tau_2\tau_3\tau_4\tau_5\tau_6\tau_7\tau_8}\int d\mathbf{K}\int d\mathbf{k}\int d\mathbf{k}'\int d\mathbf{K}'\int d\mathbf{k}''\int d\mathbf{k}'''$$
$$\times (\mathbf{k}\sigma_1\tau_1\sigma_2\tau_2|\delta U_\lambda|\mathbf{k}'\sigma_3\tau_3\sigma_4\tau_4)(\mathbf{k}''\sigma_5\tau_5\sigma_6\tau_6|\delta U_\lambda^\dagger|\mathbf{k}'''\sigma_7\tau_7\sigma_8\tau_8)\delta_{\sigma_4\sigma_6}\delta_{\sigma_3\sigma}\delta_{\sigma\sigma_5}\delta_{\tau_4\tau_6}\delta_{\tau_3\tau}\delta_{\tau\tau_5}$$
$$\times \delta(\mathbf{K}/2-\mathbf{k}'-\mathbf{K}'/2+\mathbf{k}'')\delta(\mathbf{K}/2+\mathbf{k}'-\mathbf{q})\delta(\mathbf{q}-\mathbf{K}'/2-\mathbf{k}'')$$
$$\times a^\dagger_{\frac{1}{2}\mathbf{K}+\mathbf{k}\sigma_1\tau_1} a^\dagger_{\frac{1}{2}\mathbf{K}-\mathbf{k}\sigma_2\tau_2} a_{\frac{1}{2}\mathbf{K}'-\mathbf{k}'''\sigma_8\tau_8} a_{\frac{1}{2}\mathbf{K}'+\mathbf{k}'''\sigma_7\tau_7}$$
$$= \frac{1}{4}\sum_{\sigma_1\sigma_2\sigma_3\sigma_4\sigma\sigma'}\ \sum_{\tau_1\tau_2\tau_3\tau_4\tau'}\int d\mathbf{K}\int d\mathbf{k}\int d\mathbf{k}'$$
$$\times (\mathbf{k}\sigma_1\tau_1\sigma_2\tau_2|\delta U_\lambda|\mathbf{q}-\mathbf{K}/2\sigma\tau\sigma'\tau')(\mathbf{q}-\mathbf{K}/2\sigma\tau\sigma'\tau'|\delta U_\lambda^\dagger|\mathbf{k}'\sigma_3\tau_3\sigma_4\tau_4)$$
$$\times a^\dagger_{\frac{1}{2}\mathbf{K}+\mathbf{k}\sigma_1\tau_1} a^\dagger_{\frac{1}{2}\mathbf{K}-\mathbf{k}\sigma_2\tau_2} a_{\frac{1}{2}\mathbf{K}-\mathbf{k}'\sigma_4\tau_4} a_{\frac{1}{2}\mathbf{K}+\mathbf{k}'\sigma_3\tau_3}, \tag{9}$$

where again we relabeled in the $\delta U_\lambda^\dagger$ term for a simpler expression.

## B. Woods-Saxon orbitals

To evaluate matrix elements with respect to $A$-nucleon ground states, we replace the fully evolved ground state $\left|\Psi_0^A(\lambda)\right\rangle$ by a single Slater determinant of Woods-Saxon orbitals

$$\left|\Psi_0^A(\lambda)\right\rangle \to \prod_{\alpha<\mathrm{F}} a_\alpha^\dagger \left|0\right\rangle , \tag{10}$$

where the indices run over occupied single-particle (s.p.) states $\alpha \equiv (n_\alpha,\, l_\alpha,\, j_\alpha,\, m_{j_\alpha},\, m_{t_\alpha})$ with spin $s_\alpha = 1/2$ and isospin $t_\alpha = 1/2$, and F refers to the Fermi surface. The quantum numbers denoted by $\alpha$ refer to the principal quantum number, orbital angular momentum, total angular momentum, total angular momentum projection, and isospin projection, respectively. We transform the creation and annihilation operators from the plane-wave basis to the s.p. basis of Woods-Saxon orbitals using

$$a_{\mathbf{k}\sigma\tau} = \sum_\alpha \psi_\alpha(\mathbf{k};\sigma,\tau)\, a_\alpha, \tag{11}$$

where $\psi_\alpha(\mathbf{k};\sigma,\tau)$ is a s.p. wave function with respect to orbital $\alpha$. The s.p. wave function is given by

$$\psi_\alpha(\mathbf{k};\sigma,\tau) = \phi_{n_\alpha l_\alpha j_\alpha m_{t_\alpha}}(k)\, \mathcal{Y}_{l_\alpha 1/2 j_\alpha m_{j_\alpha}}(\hat{k};\sigma)\, \chi^{(\tau)}_{m_{t_\alpha}}, \tag{12}$$

where

$$\mathcal{Y}_{l_\alpha 1/2 j_\alpha m_{j_\alpha}}(\hat{k};\sigma) = \sum_{m_{l_\alpha}} \sum_{m_{s_\alpha}} \langle j_\alpha m_{j_\alpha} | l_\alpha m_{l_\alpha} 1/2\, m_{s_\alpha}\rangle\; Y_{l_\alpha m_{l_\alpha}}(\hat{k})\, \eta^{(\sigma)}_{m_{s_\alpha}}, \tag{13}$$

and

$$\phi_\alpha(k) = i^{-l_\alpha} \sqrt{\frac{2}{\pi}} \int_0^\infty dr\, r\, j_{l_\alpha}(kr)\, u_\alpha(r). \tag{14}$$

where $j_{l_\alpha}$ is a spherical Bessel function. The functions $\eta_{m_{s_\alpha}}$ and $\chi_{m_{t_\alpha}}$ are spinors and isospinors for spin $s_\alpha = 1/2$ and isospin $t_\alpha = 1/2$, respectively. The radial s.p. wave functions $u_\alpha(r)$ are obtained from the Woods-Saxon potential.

Next we will substitute Eq. (11) into each of the four terms evaluated previously:

$$\widehat{I}\widehat{n}^\tau(\mathbf{q})\widehat{I} = \sum_\sigma \sum_{\alpha\beta} \psi_\alpha^\dagger(\mathbf{q};\sigma,\tau)\psi_\beta(\mathbf{q};\sigma,\tau) a_\alpha^\dagger a_\beta, \tag{15}$$

$$\begin{aligned}\delta\widehat{U}_\lambda \widehat{n}^\tau(\mathbf{q})\widehat{I} = \frac{1}{2} \sum_{\sigma_1\sigma_2\sigma\sigma'} \sum_{\tau_1\tau_2\tau'} \sum_{\alpha\beta\gamma\delta} \int d\mathbf{K} \int d\mathbf{k} (\mathbf{k}\sigma_1\tau_1\sigma_2\tau_2 | \delta U_\lambda | \mathbf{q} - \mathbf{K}/2\sigma\tau\sigma'\tau') \\ \times \psi_\alpha^\dagger(\mathbf{K}/2+\mathbf{k};\sigma_1,\tau_1)\psi_\beta^\dagger(\mathbf{K}/2-\mathbf{k};\sigma_2,\tau_2)\psi_\delta(\mathbf{K}-\mathbf{q};\sigma',\tau')\psi_\gamma(\mathbf{q};\sigma,\tau) a_\alpha^\dagger a_\beta^\dagger a_\delta a_\gamma,\end{aligned} \tag{16}$$

$$
\begin{aligned}
\widehat{I}\widehat{n}^{\tau}(\mathbf{q})\delta\widehat{U}^{\dagger}_{\lambda} \equiv \frac{1}{2}& \sum_{\sigma_1\sigma_2\sigma\sigma'}\sum_{\tau_1\tau_2\tau'}\sum_{\alpha\beta\gamma\delta}\int d\mathbf{K}\int d\mathbf{k}(\mathbf{q}-\mathbf{K}/2\sigma\tau\sigma'\tau'|\delta U^{\dagger}_{\lambda}|\mathbf{k}\sigma_1\tau_1\sigma_2\tau_2) \\
&\times \psi^{\dagger}_{\gamma}(\mathbf{q};\sigma,\tau)\psi^{\dagger}_{\delta}(\mathbf{K}-\mathbf{q};\sigma',\tau')\psi_{\beta}(\mathbf{K}/2-\mathbf{k};\sigma_2,\tau_2)\psi_{\alpha}(\mathbf{K}/2+\mathbf{k};\sigma_1,\tau_1)a^{\dagger}_{\gamma}a^{\dagger}_{\delta}a_{\beta}a_{\alpha},
\end{aligned}
\tag{17}
$$

$$
\begin{aligned}
\delta\widehat{U}_{\lambda}\widehat{n}^{\tau}(\mathbf{q})\delta\widehat{U}^{\dagger}_{\lambda} = \frac{1}{4}& \sum_{\sigma_1\sigma_2\sigma_3\sigma_4\sigma\sigma'}\sum_{\tau_1\tau_2\tau_3\tau_4\tau'}\sum_{\alpha\beta\gamma\delta}\int d\mathbf{K}\int d\mathbf{k}\int d\mathbf{k}' \\
&\times (\mathbf{k}\sigma_1\tau_1\sigma_2\tau_2|\delta U_{\lambda}|\mathbf{q}-\mathbf{K}/2\sigma\tau\sigma'\tau')(\mathbf{q}-\mathbf{K}/2\sigma\tau\sigma'\tau'|\delta U^{\dagger}_{\lambda}|\mathbf{k}'\sigma_3\tau_3\sigma_4\tau_4) \\
&\times \psi^{\dagger}_{\alpha}(\mathbf{K}/2+\mathbf{k};\sigma_1,\tau_1)\psi^{\dagger}_{\beta}(\mathbf{K}/2-\mathbf{k};\sigma_2,\tau_2)\psi_{\delta}(\mathbf{K}/2-\mathbf{k}';\sigma_4,\tau_4)\psi_{\gamma}(\mathbf{K}/2+\mathbf{k}';\sigma_3,\tau_3) \\
&\times a^{\dagger}_{\alpha}a^{\dagger}_{\beta}a_{\delta}a_{\gamma},
\end{aligned}
\tag{18}
$$

We evaluate matrix elements of the evolved operator with respect to $\left|\Psi^{A}_{0}(\lambda)\right\rangle$ where contractions are given by

$$
\overbracket{a^{\dagger}_{\alpha}a_{\beta}} = \left\langle\Psi^{A}_{0}(\lambda)\middle|a^{\dagger}_{\alpha}a_{\beta}\middle|\Psi^{A}_{0}(\lambda)\right\rangle = \delta_{\alpha\beta}, \tag{19}
$$

for $\alpha, \beta < \mathrm{F}$ and zero otherwise:

$$
\begin{aligned}
\left\langle\Psi^{A}_{0}(\lambda)\middle|\widehat{I}\widehat{n}^{\tau}(\mathbf{q})\widehat{I}\middle|\Psi^{A}_{0}(\lambda)\right\rangle &= \sum_{\sigma}\sum_{\alpha\beta}\psi^{\dagger}_{\alpha}(\mathbf{q};\sigma,\tau)\psi_{\beta}(\mathbf{q};\sigma,\tau)\overbracket{a^{\dagger}_{\alpha}a_{\beta}} \\
&= \sum_{\sigma}\sum_{\alpha\beta<\mathrm{F}}\psi^{\dagger}_{\alpha}(\mathbf{q};\sigma,\tau)\psi_{\beta}(\mathbf{q};\sigma,\tau)\delta_{\alpha\beta} \\
&= \sum_{\sigma}\sum_{\alpha<\mathrm{F}}\left|\psi_{\alpha}(\mathbf{q};\sigma,\tau)\right|^{2},
\end{aligned}
\tag{20}
$$

$$
\begin{aligned}
&\left\langle\Psi^{A}_{0}(\lambda)\middle|\delta\widehat{U}_{\lambda}\widehat{n}^{\tau}(\mathbf{q})\widehat{I}\middle|\Psi^{A}_{0}(\lambda)\right\rangle \\
&\quad= \frac{1}{2}\sum_{\sigma_1\sigma_2\sigma\sigma'}\sum_{\tau_1\tau_2\tau'}\sum_{\alpha\beta\gamma\delta}\int d\mathbf{K}\int d\mathbf{k}(\mathbf{k}\sigma_1\tau_1\sigma_2\tau_2|\delta U_{\lambda}|\mathbf{q}-\mathbf{K}/2\sigma\tau\sigma'\tau')\psi^{\dagger}_{\alpha}(\mathbf{K}/2+\mathbf{k};\sigma_1,\tau_1) \\
&\quad\times \psi^{\dagger}_{\beta}(\mathbf{K}/2-\mathbf{k};\sigma_2,\tau_2)\psi_{\delta}(\mathbf{K}-\mathbf{q};\sigma',\tau')\psi_{\gamma}(\mathbf{q};\sigma,\tau)\big(\overbracket{a^{\dagger}_{\alpha}a_{\gamma}}\overbracket{a^{\dagger}_{\beta}a_{\delta}}-\overbracket{a^{\dagger}_{\alpha}a_{\delta}}\overbracket{a^{\dagger}_{\beta}a_{\gamma}}\big) \\
&\quad= \frac{1}{2}\sum_{\sigma_1\sigma_2\sigma\sigma'}\sum_{\tau_1\tau_2\tau'}\sum_{\alpha\beta\gamma\delta<\mathrm{F}}\int d\mathbf{K}\int d\mathbf{k}(\mathbf{k}\sigma_1\tau_1\sigma_2\tau_2|\delta U_{\lambda}|\mathbf{q}-\mathbf{K}/2\sigma\tau\sigma'\tau')\psi^{\dagger}_{\alpha}(\mathbf{K}/2+\mathbf{k};\sigma_1,\tau_1) \\
&\quad\times \psi^{\dagger}_{\beta}(\mathbf{K}/2-\mathbf{k};\sigma_2,\tau_2)\psi_{\delta}(\mathbf{K}-\mathbf{q};\sigma',\tau')\psi_{\gamma}(\mathbf{q};\sigma,\tau)\big(\delta_{\alpha\gamma}\delta_{\beta\delta}-\delta_{\alpha\delta}\delta_{\beta\gamma}\big) \\
&\quad= \frac{1}{2}\sum_{\sigma_1\sigma_2\sigma\sigma'}\sum_{\tau_1\tau_2\tau'}\sum_{\alpha\beta<\mathrm{F}}\int d\mathbf{K}\int d\mathbf{k}(\mathbf{k}\sigma_1\tau_1\sigma_2\tau_2|\delta U_{\lambda}|\mathbf{q}-\mathbf{K}/2\sigma\tau\sigma'\tau')\psi^{\dagger}_{\alpha}(\mathbf{K}/2+\mathbf{k};\sigma_1,\tau_1) \\
&\quad\times \psi^{\dagger}_{\beta}(\mathbf{K}/2-\mathbf{k};\sigma_2,\tau_2)\big(\psi_{\beta}(\mathbf{K}-\mathbf{q};\sigma',\tau')\psi_{\alpha}(\mathbf{q};\sigma,\tau)-\psi_{\alpha}(\mathbf{K}-\mathbf{q};\sigma',\tau')\psi_{\beta}(\mathbf{q};\sigma,\tau)\big),
\end{aligned}
\tag{21}
$$

$$
\begin{aligned}
&\big\langle \Psi_0^A(\lambda)\big|\widehat{I}\widehat{n}^\tau(\mathbf{q})\delta\widehat{U}_\lambda^\dagger\big|\Psi_0^A(\lambda)\big\rangle \\
&\quad = \frac{1}{2}\sum_{\sigma_1\sigma_2\sigma\sigma'}\sum_{\tau_1\tau_2\tau'}\sum_{\alpha\beta<\mathrm{F}}\int d\mathbf{K}\int d\mathbf{k}(\mathbf{q}-\mathbf{K}/2\sigma\tau\sigma'\tau'|\delta U_\lambda^\dagger|\mathbf{k}\sigma_1\tau_1\sigma_2\tau_2)\psi_\alpha(\mathbf{K}/2+\mathbf{k};\sigma_1,\tau_1) \\
&\qquad \times \psi_\beta(\mathbf{K}/2-\mathbf{k};\sigma_2,\tau_2)\big(\psi_\beta^\dagger(\mathbf{K}-\mathbf{q};\sigma',\tau')\psi_\alpha^\dagger(\mathbf{q};\sigma,\tau)-\psi_\alpha^\dagger(\mathbf{K}-\mathbf{q};\sigma',\tau')\psi_\beta^\dagger(\mathbf{q};\sigma,\tau)\big),
\end{aligned}
\tag{22}
$$

$$
\begin{aligned}
&\big\langle \Psi_0^A(\lambda)\big|\delta\widehat{U}_\lambda\widehat{n}^\tau(\mathbf{q})\delta\widehat{U}_\lambda^\dagger\big|\Psi_0^A(\lambda)\big\rangle \\
&\quad = \frac{1}{4}\sum_{\sigma_1\sigma_2\sigma_3\sigma_4\sigma\sigma'}\sum_{\tau_1\tau_2\tau_3\tau_4\tau'}\sum_{\alpha\beta\gamma\delta}\int d\mathbf{K}\int d\mathbf{k}\int d\mathbf{k}'(\mathbf{k}\sigma_1\tau_1\sigma_2\tau_2|\delta U_\lambda|\mathbf{q}-\mathbf{K}/2\sigma\tau\sigma'\tau') \\
&\qquad \times (\mathbf{q}-\mathbf{K}/2\sigma\tau\sigma'\tau'|\delta U_\lambda^\dagger|\mathbf{k}'\sigma_3\tau_3\sigma_4\tau_4)\psi_\alpha^\dagger(\mathbf{K}/2+\mathbf{k};\sigma_1,\tau_1)\psi_\beta^\dagger(\mathbf{K}/2-\mathbf{k};\sigma_2,\tau_2) \\
&\qquad \times \psi_\delta(\mathbf{K}/2-\mathbf{k}';\sigma_4,\tau_4)\psi_\gamma(\mathbf{K}/2+\mathbf{k}';\sigma_3,\tau_3)\big(\overbracket{a_\alpha^\dagger a_\gamma}\overbracket{a_\beta^\dagger a_\delta}-\overbracket{a_\alpha^\dagger a_\delta}\overbracket{a_\beta^\dagger a_\gamma}\big) \\
&\quad = \frac{1}{4}\sum_{\sigma_1\sigma_2\sigma_3\sigma_4\sigma\sigma'}\sum_{\tau_1\tau_2\tau_3\tau_4\tau'}\sum_{\alpha\beta\gamma\delta}\int d\mathbf{K}\int d\mathbf{k}\int d\mathbf{k}'(\mathbf{k}\sigma_1\tau_1\sigma_2\tau_2|\delta U_\lambda|\mathbf{q}-\mathbf{K}/2\sigma\tau\sigma'\tau') \\
&\qquad \times (\mathbf{q}-\mathbf{K}/2\sigma\tau\sigma'\tau'|\delta U_\lambda^\dagger|\mathbf{k}'\sigma_3\tau_3\sigma_4\tau_4)\psi_\alpha^\dagger(\mathbf{K}/2+\mathbf{k};\sigma_1,\tau_1)\psi_\beta^\dagger(\mathbf{K}/2-\mathbf{k};\sigma_2,\tau_2) \\
&\qquad \times \psi_\delta(\mathbf{K}/2-\mathbf{k}';\sigma_4,\tau_4)\psi_\gamma(\mathbf{K}/2+\mathbf{k}';\sigma_3,\tau_3)\big(\delta_{\alpha\gamma}\delta_{\beta\delta}-\delta_{\alpha\delta}\delta_{\beta\gamma}\big) \\
&\quad = \frac{1}{4}\sum_{\sigma_1\sigma_2\sigma_3\sigma_4\sigma\sigma'}\sum_{\tau_1\tau_2\tau_3\tau_4\tau'}\sum_{\alpha\beta<\mathrm{F}}\int d\mathbf{K}\int d\mathbf{k}\int d\mathbf{k}'(\mathbf{k}\sigma_1\tau_1\sigma_2\tau_2|\delta U_\lambda|\mathbf{q}-\mathbf{K}/2\sigma\tau\sigma'\tau') \\
&\qquad \times (\mathbf{q}-\mathbf{K}/2\sigma\tau\sigma'\tau'|\delta U_\lambda^\dagger|\mathbf{k}'\sigma_3\tau_3\sigma_4\tau_4)\psi_\alpha^\dagger(\mathbf{K}/2+\mathbf{k};\sigma_1,\tau_1)\psi_\beta^\dagger(\mathbf{K}/2-\mathbf{k};\sigma_2,\tau_2) \\
&\qquad \times \big(\psi_\beta(\mathbf{K}/2-\mathbf{k}';\sigma_4,\tau_4)\psi_\alpha(\mathbf{K}/2+\mathbf{k}';\sigma_3,\tau_3)-\psi_\alpha(\mathbf{K}/2-\mathbf{k}';\sigma_4,\tau_4)\psi_\beta(\mathbf{K}/2+\mathbf{k}';\sigma_3,\tau_3)\big).
\end{aligned}
\tag{23}
$$

### C. Partial wave expansion

Lastly we expand the $\delta U$ and $\delta U^\dagger$ plane-wave matrix elements in the relative momentum partial wave basis. To do this, we use the following expansion

$$
\begin{aligned}
|\mathbf{K}\mathbf{k}\sigma_1\tau_1\sigma_2\tau_2\rangle = \frac{1}{\sqrt{2}}\sum_{SM_S}\sum_{LM_L}\sum_{JM_J}\sum_{TM_T}\langle\sigma_1\sigma_2|SM_S\rangle\langle\tau_1\tau_2|TM_T\rangle\sqrt{\frac{2}{\pi}}Y_{LM_L}^*(\Omega_\mathbf{k}) \\
\times\langle LM_LSM_S|JM_J\rangle\,[1-(-1)^{L+S+T}]|\mathbf{K}k(LS)JM_JTM_T).
\end{aligned}
\tag{24}
$$

Here $L$ and $J$ are the total orbital angular momentum and total angular momentum, respectively, associated with the relative momentum $k$. $S$ is the total spin and $T$ is the total isospin. Note, the LHS of Eq. (24) is already written in terms of relative momenta $\mathbf{k}$ and

center-of-mass (CoM) momenta $\mathbf{K}$, where $\mathbf{k} \equiv \frac{1}{2}(\mathbf{k}_1 - \mathbf{k}_2)$, $\mathbf{K} \equiv \mathbf{k}_1 + \mathbf{k}_2$, and $\mathbf{k}_1$ and $\mathbf{k}_2$ are s.p. vector momenta. Furthermore, the matrix elements of $\delta U$ do not depend on the CoM momentum $\mathbf{K}$ as seen in Eq. (4). We apply Eq. (24) to the $\delta U$ matrix elements to obtain

$$
\begin{aligned}
&(\mathbf{k}\sigma_1\tau_1\sigma_2\tau_2|\delta U_\lambda|\mathbf{k}'\sigma_3\tau_3\sigma_4\tau_4) \\
&\quad = \frac{1}{2}\frac{2}{\pi} \sum_{SM_SM'_S} \sum_{LM_LL'M'_L} \sum_{JM_J} \sum_{TM_T} \langle\sigma_1\sigma_2|SM_S\rangle \langle SM'_S|\sigma_3\sigma_4\rangle \langle\tau_1\tau_2|TM_T\rangle \langle TM_T|\tau_3\tau_4\rangle \\
&\quad \times Y_{LM_L}(\Omega_{\mathbf{k}}) Y^*_{L'M'_L}(\Omega_{\mathbf{k}'}) \langle LM_LSM_S|JM_J\rangle \langle JM_J|L'M'_LSM'_S\rangle \left[1-(-1)^{L+S+T}\right] \\
&\quad \times \left[1-(-1)^{L'+S+T}\right] (k(LS)JM_JTM_T|\delta U_\lambda|k'(L'S)JM_JTM_T). \qquad (25)
\end{aligned}
$$

There are no $S'$, $J'$, $M'_J$, $T'$, or $M'_T$ because the $\delta U$ matrix elements are diagonal in total spin, total angular momentum, total angular momentum projection, total isospin, and total isospin projection. The analogous expression for $\delta U^\dagger$ follows similarly. Substituting these expansions into Eqs. (20), (21), (22), and (23), and combining gives the full momentum distribution.


[1] I. Angeli and K. Marinova, Atomic Data and Nuclear Data Tables **99**, 69 (2013).

[2] A. J. Tropiano, S. K. Bogner, and R. J. Furnstahl, Phys. Rev. C **104**, 034311 (2021), arXiv:2105.13936 [nucl-th].
